# Supplementary material for: Zeptosecond Angular Streak Camera
Source: arXiv:2206.00581 source file (2022-06-01)
Supplement: Supplementary file 1 [file streak_supp.pdf]

# Supplemental Material: Zeptosecond Angular Streak Camera


Hongcheng Ni,[1,2,3,4] Stefan Donsa,[2] Xiaochun Gong,[1,3] Kiyoshi Ueda,[1,5] Jian Wu,[1,3,4,6] and Joachim Burgdörfer[2]

[1]*State Key Laboratory of Precision Spectroscopy, East China Normal University, Shanghai 200241, China*
[2]*Institute for Theoretical Physics, Vienna University of Technology, 1040 Vienna, Austria*
[3]*Collaborative Innovation Center of Extreme Optics, Shanxi University, Taiyuan, Shanxi 030006, China*
[4]*NYU-ECNU Joint Institute of Physics, New York University at Shanghai, Shanghai 200062, China*
[5]*Department of Chemistry, Tohoku University, Sendai 980-8578, Japan*
[6]*CAS Center for Excellence in Ultra-intense Laser Science, Shanghai 201800, China*


In this work, the numerical simulation is carried out using the time-dependent Schrödinger equation (TDSE), which is written in the dipole approximation as

$$i\frac{\partial}{\partial t}\psi = \left[\frac{\boldsymbol{p}^2}{2} - \frac{1}{r} + \boldsymbol{r}\cdot\boldsymbol{F}(t)\right]\psi, \tag{S1}$$

where $\boldsymbol{p}$ is the momentum operator, $\boldsymbol{r}$ is the position operator, $\boldsymbol{F}(t)$ is the combined electric field vector of the laser field composed of an XUV and an IR pulse, which are both defined in terms of their vector potential with $\boldsymbol{F}(t) = -\boldsymbol{A}'(t)$. The TDSE is solved using the well-established pseudospectral method. The energy eigenstates are obtained from the field-free Hamiltonian in a basis of the finite-element discrete variable representation, and the time propagation is carried out using a split-operator method where the evolution in the Coulomb field is carried out in the energy domain and the evolution within the laser field is done in the coordinate space. To compute the photoelectron momentum distribution, we project the wave function onto the Coulomb wave after the laser pulse is over.

The projected two-dimensional photoelectron momentum in the polarization plane is distributed along a center-displaced circle. Thereby, the location of the expected radial momentum is given by

$$\langle p(\phi)\rangle = \sqrt{p_0^2 - k_0^2\sin^2(\phi-\phi_0)} + k_0\cos(\phi-\phi_0) \tag{S2}$$

$$\approx p_0 + k_0\cos(\phi-\phi_0), \tag{S3}$$

where we have used $k_0 \ll p_0$ for a typical streaking scenario allowing to drop the $k_0^2$ term. Here, $p_0$ is the mean photoelectron momentum in the absence of the streaking field, $k_0$ is the magnitude of the IR-field-induced displacement of the photoelectron momentum distribution, and $\phi_0$ is the streaking angle. The streaking angle $\phi_0$ is extracted by fitting the expected radial momentum to this equation.

In general, the streaking trace can have a different angular frequency than that of the original streaking pulse. This fact becomes obvious from the context of the present zeptosecond angular streak camera with a circular streaking pulse, which has a simple streaking trace of a straight line, whose slope is the angular frequency:

$$\phi_0(\tau) = \omega_s(\tau + t_s). \tag{S4}$$

As shown in Fig. S1, the numerical streaking trace has a slightly smaller slope than $\omega_{\mathrm{IR}}$. Instead, the numerical streaking trace has a slope that almost coincides with the convoluted angular frequency

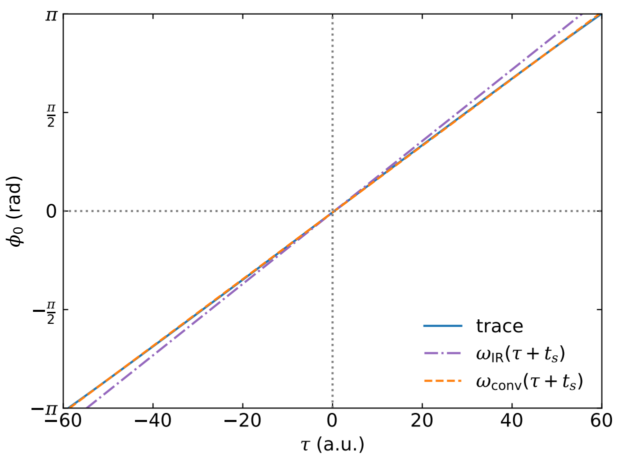


FIG. S1. The streaking trace (blue solid line) of the zeptosecond angular streak camera employing an XUV pump pulse with a central wavelength of 20 nm and a circular streaking pulse. Its slope is compared to the original angular frequency of the streaking pulse $\omega_{\mathrm{IR}}$ (purple dash-dotted line) and the convoluted angular frequency [Eq. (S5)].

$$\omega_{\mathrm{conv}} = \frac{1}{1+(\tau_{\mathrm{XUV}}/\tau_{\mathrm{IR}})^2/2}\,\omega_{\mathrm{IR}}. \tag{S5}$$

To derive the convoluted angular frequency [Eq. (S5)], we note that photoionization, namely single-photon ionization, is a linear process, where the ionization rate $P(t)$ is proportional to the field intensity. This ionization rate $P(t)$ is the input signal to be streaked in the $x$ and $y$ directions, while the output signal is the convolution of the input signal with the system impulse response, or, the streaking process, so that

$$\Delta p_x = [P*(-A_{\mathrm{IR},x})](t), \tag{S6}$$

$$\Delta p_y = [P*(-A_{\mathrm{IR},y})](t), \tag{S7}$$

leading to the streaking angle

$$\Delta\phi = \arctan\left(\frac{\Delta p_y}{\Delta p_x}\right) = \arctan\left\{\frac{[P*(-A_{\mathrm{IR},y})](t)}{[P*(-A_{\mathrm{IR},x})](t)}\right\}. \tag{S8}$$

In the main text, we have used a field envelope of $\cos^4$ shape for the purpose of convenient numerical computation. To ob-

tain an analytical expression for the convoluted angular frequency here, however, we employ for simplicity a Gaussian-shaped envelope. Since only the ratio of the XUV and IR pulse durations matters, the particular choice of the envelope shape is not critical. Consequently, the photoionization rate may be written as

$$P(t) \sim \exp\left\{-\frac{2t^2\ln(4)}{\tau_{\rm XUV}^2}\right\}. \tag{S9}$$

The streaking pulse can be rewritten as

$$A_{{\rm IR},x}(t) \sim -\exp\left\{-\frac{t^2\ln(4)}{\tau_{\rm IR}^2}\right\}\cos(\omega_{\rm IR}t), \tag{S10}$$

$$A_{{\rm IR},y}(t) \sim -\varepsilon\exp\left\{-\frac{t^2\ln(4)}{\tau_{\rm IR}^2}\right\}\sin(\omega_{\rm IR}t). \tag{S11}$$

Inserting these expressions into Eq. (S8), we have

$$\Delta\phi = \arctan\left[\varepsilon\tan(\omega_{\rm conv}t)\right], \tag{S12}$$

where

$$\omega_{\rm conv} = \frac{1}{1+(\tau_{\rm XUV}/\tau_{\rm IR})^2/2}\omega_{\rm IR}. \tag{S13}$$

It is easy to further extend this observation to multiphoton ionization processes. For an $n$-photon ionization in general, the convoluted angular frequency of the streaking trace is

$$\omega_{\rm conv}^{(n)} = \frac{1}{1+(\tau_{\rm XUV}/\tau_{\rm IR})^2/2n}\omega_{\rm IR}. \tag{S14}$$
